# Supplementary material for: RealDexUMI: A Wearable Universal Manipulation Interface for Dexterous Robot Learning
Source: arXiv:2606.06033 source file (2026-06-06)
Supplement: Supplementary file 1 [file table_experiment_appendix.tex]

\begin{table}[t]
\centering
\small
\setlength{\tabcolsep}{3.5pt}

\caption{
Cumulative subgoal completion for multi-stage tasks.
Each entry reports the number of trials that reach the corresponding subgoal while completing all previous subgoals in the same rollout.
}
\label{tab:subgoal_breakdown}
\begin{tabular}{
L{2.4cm}
C{2.2cm}
C{2.2cm}
C{2.2cm}
C{2.2cm}
}
\toprule
Task & Subgoal 1 & Subgoal 2 & Subgoal 3 & Subgoal 4 \\
\midrule
Drawer stowing
& Open drawer
\newline 20/20
& Pick cube
\newline 18/20
& Close drawer
\newline 17/20
& -- \\
\midrule
Tea transfer
& Grasp tweezers
\newline 17/20
& Pick tea leaves
\newline 16/20
& Place tea in cup
\newline 16/20
& -- \\
\midrule
Egg transfer
& Open carton
\newline 15/20
& Pick egg
\newline 14/20
& Place egg in pot
\newline 14/20
& -- \\
\midrule
Multi-object grasping
& Grasp first object
\newline 20/20
& Grasp second object
\newline 20/20
& -- 
& -- \\
\midrule
Bimanual package scanning
& Pick scanner
\newline 18/20
& Pick package
\newline 18/20
& Scan package
\newline 18/20
& Drop package in box
\newline 18/20 \\
\bottomrule
\end{tabular}
\end{table}

\paragraph{Subgoal analysis.}
Table~\ref{tab:subgoal_breakdown} reports cumulative subgoal completion for the multi-stage tasks.
Most failures occur at the first contact-sensitive stage of each long-horizon sequence.
For drawer stowing, the policy reliably opens the drawer, while failures mainly arise during cube retrieval and final closure.
For tea and egg transfer, later subgoals do not introduce additional failures once the object is successfully picked, indicating that grasp acquisition is the main bottleneck.
Multi-object grasping completes both sequential grasps in all trials, while bimanual package scanning shows no additional degradation after the scanner and package are grasped.
These results indicate that RealDexUMI policies can maintain sequential progress once reliable contact is established, with failures concentrated in fine contact acquisition rather than later execution.
